# Supplementary material for: Detection of zeptojoule microwave pulses using electrothermal feedback in proximity-induced Josephson junctions
Source: arXiv:1512.07235 ancillary file (2016-06-14)
Supplement: Supplementary file 1 [file zJ-detection_supplemental.pdf]

# Detection of zeptojoule microwave pulses using electrothermal feedback in proximity-induced Josephson junctions: Supplemental material


J. Govenius,* R. E. Lake, K. Y. Tan, and M. Möttönen

*QCD Labs, COMP Centre of Excellence, Department of Applied Physics, Aalto University, P.O. Box 13500, FIN-00076 Aalto, Finland*


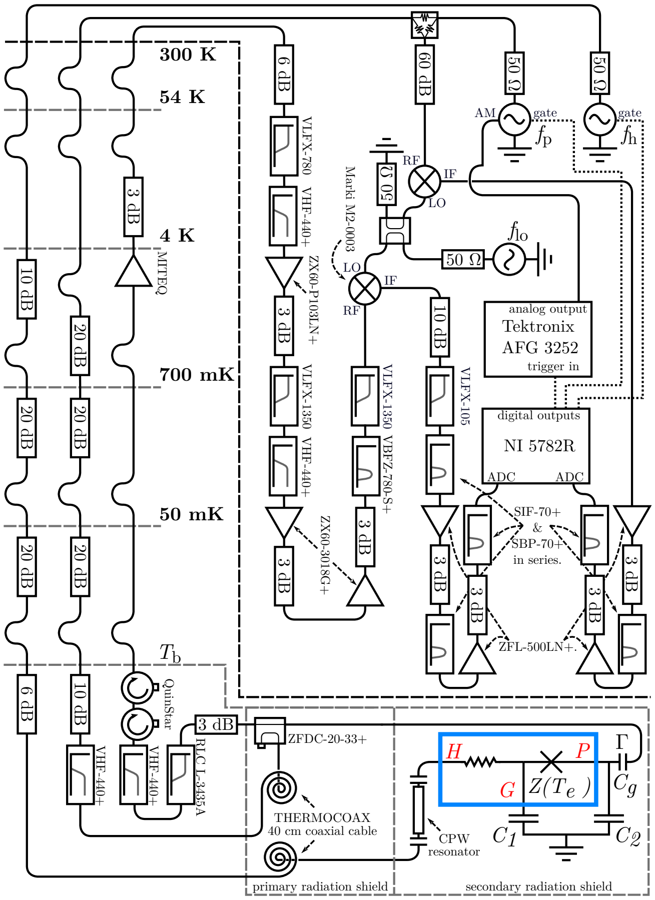


Figure S1. Detailed diagram of the experimental setup. The on-chip coplanar waveguide (CPW) resonator, used as a bandpass filter, and the on-chip capacitors inside the secondary radiation shield are shown in Fig. S2. The blue rectangle denotes the nanostructure shown in Fig. 1(b). The filter, coupler, and amplifier model numbers refer to Mini-Circuits models, except for the RLC L-3435A low-pass filter.

## I. EXPERIMENTAL SETUP

Figure S1 shows a detailed diagram of the analog parts of the experimental setup. The heater generator is connected to lead $H$ via various attenuators and filters. The probe generator output is split into two separate paths, one of which goes through the cryostat and reflects off of the detector before amplification, down-conversion, and digitization. We call the transmission coefficient through this path $S_{21}$. The second path is used as a phase reference for determining $\arg(S_{21})$. The local oscillator frequency is $f_{lo} = f_p - 70.3125$ MHz. Real-time digital signal processing and pulsing of the generators is performed by a custom field-programmable gate array (NI PXIE-7962R) connected to the transceiver (NI 5782R). The real-time digital processing includes digital down-conversion, moving average filtering with down sampling, and, in some experiments, ensemble averaging over many repetitions of the same pulse sequence.

The cryogenic amplifier from Miteq has a noise temperature between 10 K and 14 K for frequencies between 100 MHz and 2 GHz (tested at 77 K). The cryogenic isolators from Quinstar are specified for the 560 MHz to 640 MHz frequency range, but are also acceptable for our purposes. That is, up to 780 MHz, they have forward (reverse) transmission better than $-3.4$ dB ($-14$ dB) each. In addition, we have placed a 3 dB attenuator between the sample and the circulators in order to suppress reflections from the circulators. This implies that, referred to the output of the directional coupler, the effective noise temperature is of the order of 100 K. In comparison, well matched circulators together with a state-of-the-art Josephson parametric amplifier, or a SQUID microstrip amplifier, would be expected to provide an effective noise temperature of the order of 100 mK. This justifies our claim that a state-of-the-art amplifier "should reduce the required averaging time by at least two orders of magnitude."

Figure S2(a) shows the on-chip components inside the secondary radiation shield. The heater (probe) input is connected the left (right) bonding pad. The meandering structure is a symmetrically coupled coplanar waveguide (CPW) resonator used as the 8.4 GHz bandpass filter also shown in Fig. 1(a). The white areas form the Nb-AlO$_x$-Al capacitors $C_1$, $C_2$, and $C_g$. The rest of the Nb parts are bonded to ground at the perimeter of the chip.

Figure S2(b) shows a projection of the complex reflection coefficient as a function of $f_h$ for $P_h = -130$ dBm, $P_p = -135$ dBm, and $T_b = 11$ mK. As expected for a symmetrically coupled CPW resonator, the heating power through the resonator is approximately Lorentzian, although the linewidth is only 49 MHz compared to 74 MHz measured for a nominally identical CPW resonator at 4.2 K [Fig. S2(c)]. We do not expect the linewidth of an externally loaded CPW resonator to change so significantly as a function of temperature. The external loading is evident from the low insertion loss on resonance in Fig. S2(c). We attribute the additional narrowing of the linewidth to imperfect impedance matching between the THERMOCOAX cable, the CPW resonator, and the load impedance provided by the detector. Note that the lower resonance frequency at 4.2 K is expected, at least qualitatively, on the basis of increased kinetic inductance.

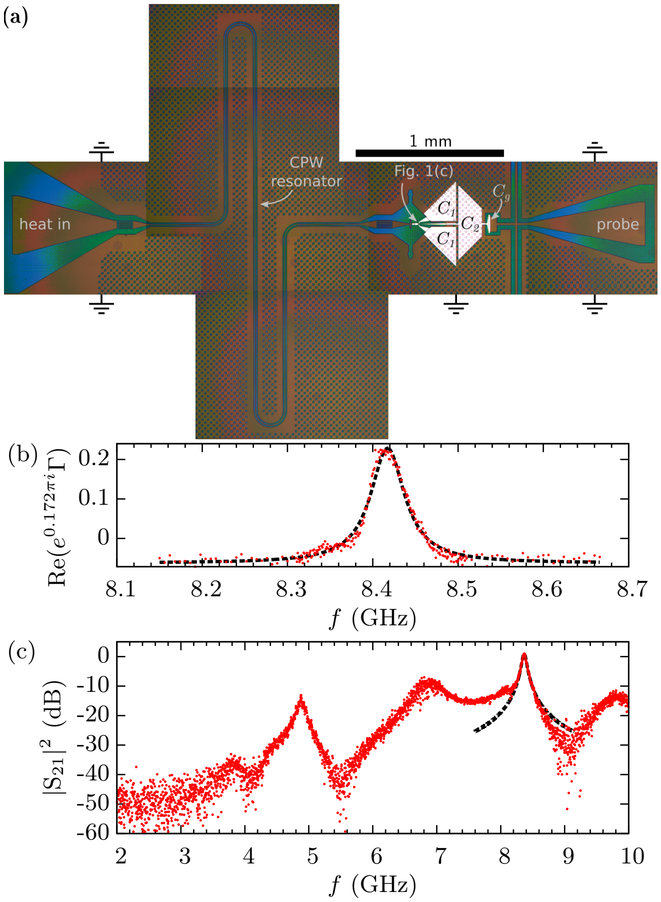


Figure S2. (a) False-color optical micrograph of the chip. The green and blue areas are high-resistivity Si (0.5 mm) with thermally grown $SiO_x$ (300 nm) and atomic layer deposited $AlO_x$ (50 nm) on top. The brown areas have sputtered Nb (200 nm) between the $SiO_x$ and $AlO_x$. The white areas have an additional evaporated Al (100 nm) top layer. The 30 nm thick evaporated $Au_xPd_{1-x}$ wire shown in Fig. 1(b) is between the $AlO_x$ and Al layers. (b) Detector response as a function of heater frequency. The dashed curve shows a Lorentzian fit with a center frequency of 8.417 GHz and a full width at half maximum (FWHM) of 49 MHz. (c) Transmission through a nominally identical test CPW resonator at 4.2 K. The dashed curve shows a Lorentzian fit with a center frequency of 8.366 GHz and a FWHM of 74 MHz.

### A. Heater power calibration

Calibration of the heater input power directly affects the main figure of merit of the detector, i.e., the single zeptojoule threshold where $F \approx 0.5$. However, calibrating the power is not straightforward because most of the components are inside the cryostat and therefore physically inaccessible when cold. Furthermore, measuring all the components in series is impractical because the total attenuation is very high (120.3 dB) at 8.413 GHz. We therefore characterize the heater input line in segments.

The first source of uncertainty is the microwave source power. The specifications for the Gigatronics 2550B we used promise an accuracy of $\pm 0.7$ dBm, which would be a conservative estimate of the error. As a more realistic estimate for the uncertainty, we use 0.3 dB. That is also the measured difference between the output powers of the Gigatronics 2550B and a freshly calibrated Rohde & Schwarz SG100A generator.

We calibrate the room-temperature cabling between the microwave source and the cryostat using a standard vector network analyzer transmission measurement. The attenuation of the room-temperature cabling is 4.27 dB with negligible uncertainty. To estimate the attenuation of the cabling inside the cryostat between room temperature and $T_b$, we measure the transmission of a pair of identical lines connected at $T_b$ with a short (4 inch) cable. From the transmission, we estimate the attenuation of each cold line to be $(9.55 \pm 0.2)$ dB, with the uncertainty based on the amplitude of the ripples in the measured transmission in the vicinity of 8.413 GHz. In addition, the three attenuators between 4 K and 50 mK contribute $(50.0 \pm 0.3)$ dB (see Fig. S1).

We calibrate the attenuation of the components between the base plate of the cryostat and the input to the secondary radiation shield by connecting them to the above mentioned calibrated pair of identical lines in a separate cooldown. We find that they contribute $(56.5 \pm 0.5)$ dB with the relatively large uncertainty coming from an unintentional periodic (21 MHz) $\pm 0.5$ dB oscillation in the measured transmission in the vicinity of 8.413 GHz. The attenuation comes mainly from the 40 cm THERMOCOAX coaxial cables used to shield the sample from high-frequency radiation.

After the THERMOCOAX cable, the signal enters the secondary radiation shield, i.e., the Cu shield covering the printed circuit board (PCB) and the Si chip. We assume that losses and unwanted reflections on the PCB and in the symmetrically coupled on-chip CPW resonator are negligible. We have confirmed that the insertion loss was negligible in a 4 K transmission measurement of an identical CPW resonator without the detector [see Fig. S2(c)].

Finally, impedance matching between the detector and the characteristic impedance $Z_0 = 50\ \Omega$ of the heater line affects the amount of heat absorbed into the nanowire. However, we consider the impedance matching an important feature of the detector itself, and therefore do not compensate for it in the calibration of the heater power. It is nevertheless interesting to estimate its magnitude. At $f_h = 8.4$ GHz, lead $G$ is effectively grounded because $|2\pi i f_h C_1|^{-1} \approx 0.2\ \Omega$. Therefore, the load impedance presented by the detector is well approximated by the impedance of the long SNS junction ($H$–$G$). Furthermore, based on dc measurements of similar junctions, we estimate the critical current of the $H$–$G$ section to be negligible (a few nA). Therefore, we may approximate the load impedance by the normal state resistance (36 Ω) of the $H$–$G$ section. This implies that the fraction of reflected power is small, roughly $|(36\ \Omega - Z_0)\,/\,(36\ \Omega + Z_0)|^2 \approx 0.03$. We estimate the normal-state resistance based on a room-temperature four-wire measurement of a long (28.6 $\mu$m) test $Au_xPd_{1-x}$ wire with the same cross-section (160 nm × 30 nm) as the $H$–$G$ section of the detector nanowire. The test wire was evaporated at the same time as the detector nanowire. We also measured the

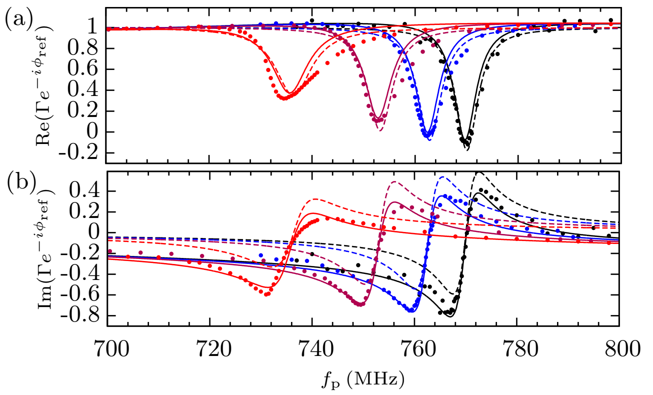


Figure S3. Measured real (a) and imaginary (b) parts of the reflection coefficient (points) as functions of probe frequency. The curves correspond to heater powers of 1.9, 66, 290, and 930 aW (from right to left). The lowest three powers are the same as in Fig. 1(c). The solid and dashed curves are fits to the circuit model with and without the phenomenological correction, respectively.

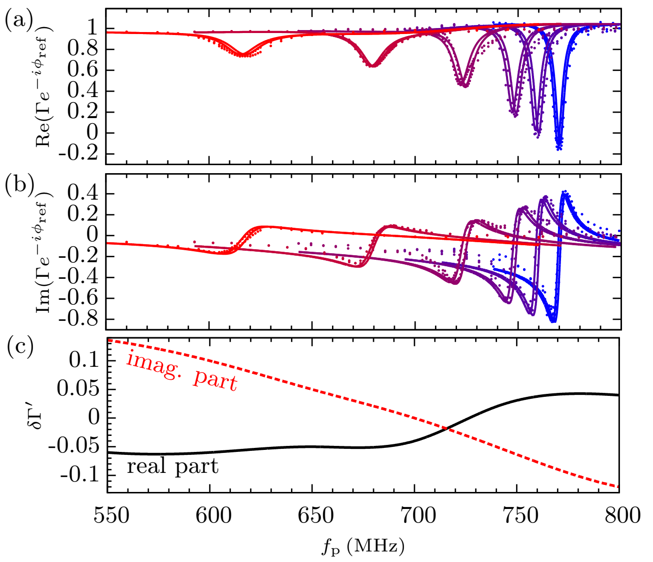


Figure S4. Measured real (a) and imaginary (b) parts of the reflection coefficient (points) as functions of probe frequency. Each pair of curves corresponds to $P_\mathrm{h} = 0$ and $P_\mathrm{h} = \delta P_\mathrm{h}$ at a fixed $T_\mathrm{b}$. The bath temperatures are 12, 80, 100, 130, 170, and 220 mK (from right to left), corresponding to $\delta P_\mathrm{h}$ of $-143.0$, $-135.0$, $-132.0$, $-127.0$, $-119.0$, and $-111.0$ dBm, respectively. The fits (solid curves) include the phenomenological correction. (c) Frequency-dependent small offset used in the fits in (a) and (b) as well as in Fig. S3.

room-temperature resistivity of the evaporated Al, 27 $\Omega$nm, using a similar Al test wire (28.6 $\mu$m $\times$ 160 nm $\times$ 100 nm).

## II. MEASUREMENT OF Γ

Here we describe how we determine Γ using the setup depicted in Fig. S1. As a first step, we measure the probe transmission coefficient $S_{21}$ for $f_\mathrm{p} = 450...898$ MHz at $T_\mathrm{b} =$ 300 mK. At this temperature, the resonance frequency of the detector is far below the measured frequency range, i.e., $Z_\mathrm{L}(T_\mathrm{b} = 300\text{ mK}) \approx (i\omega C_\mathrm{g})^{-1} + (i\omega C_2)^{-1} \approx (i\omega C_\mathrm{g})^{-1}$, where $\omega = 2\pi f_\mathrm{p}$. Therefore, this high-temperature $S_{21}$ provides a good reference for normalizing the other transmission measurement results, thereby taking into account the frequency-dependent attenuation, gain, and electrical delay of the input and output lines. More specifically, $\Gamma = e^{i\phi_\mathrm{ref}} S_{21}/S_{21}(300\text{ mK})$, assuming that the components between the circulators and port $P$ of the detector have negligible spurious reflections, and assuming that the $T_\mathrm{b}$-dependence of all the off-chip components is negligible below 300 mK. Here, $\phi_\mathrm{ref} = \arg\{[Z_\mathrm{L}(300\text{ mK}) - Z_0]/[Z_\mathrm{L}(300\text{ mK}) + Z_0]\}$ but, typically, we are not interested in the absolute phase of the reflection coefficient. Instead, we plot $|\Gamma|^2 = |S_{21}/S_{21}(300\text{ mK})|^2$ in Fig. 1(c) and $\Gamma e^{-i\phi_\mathrm{ref}} = S_{21}/S_{21}(300\text{ mK})$ in Figs. S3 and S4(a,b).

### A. Phenomenological correction to the simplified circuit model

The dashed curves in Fig. S3 show example fits using the simplified circuit model [Fig. 1(a)]. Although the fits reproduce the frequency and width of each resonance reasonably well, there is a clear systematic difference between the dashed fits and the data points, especially in $\mathrm{Im}(\Gamma e^{-i\phi_\mathrm{ref}})$ [Fig. S3(b)]. Accounting for these systematic deviations is necessary for consistent mapping of the measured Γ to the corresponding value of Δ when constructing Fig. 3(a).

We do not attempt to uniquely pinpoint which combination of approximations in the simplified circuit model leads to the observed non-ideal effects. Instead, we take a phenomenological approach and add the following small correction $\delta\Gamma$ to the Γ predicted by the simplified model [Fig. 1(a)]:

$$\delta\Gamma = e^{i\phi_\mathrm{ref}} \left[\delta\Gamma'\left(f_\mathrm{p}\right) + \delta\Gamma''\Theta\left(f_\mathrm{p}, L, R\right)\right],$$

where $\delta\Gamma'\left(f_\mathrm{p}\right)$ is the slowly-varying function shown in Fig. S4(c), $\delta\Gamma'' = 0.025 - 0.180i$, and $\Theta\left(f_\mathrm{p}, L, R\right)$ is a step-like smooth function centered at the resonance frequency. Specifically, we choose

$$\Theta\left(f_\mathrm{p}, L, R\right) = \left|\frac{1}{2} + \frac{1}{\pi}\arctan\left(-\mathrm{Im}\left[e^{-i\phi_\mathrm{ref}}\Gamma_0(L,R)\right],\right.\right.$$
$$\left.\left. + 1 - \mathrm{Re}\left[e^{-i\phi_\mathrm{ref}}\Gamma_0(L,R)\right]\right)\right|^{1/2},$$

where $\Gamma_0(L,R)$ is the prediction from the simplified model [Fig. 1(a)] and $\arctan(y,x)$ is the two-argument arc tangent function. With this choice of Θ, the step is always centered at the resonance frequency and has a width proportional to the width of the resonance. The step-height parameter $\delta\Gamma''$ and the slowly-varying offset parameter $\delta\Gamma'\left(f_\mathrm{p}\right)$ are manually chosen by optimizing the fit between the model and the off-resonant data points (i.e, points for which $\Gamma_0 e^{-i\phi_\mathrm{ref}} \approx 1$) in Fig. S3. Specifically, the offset parameter $\delta\Gamma'\left(f_\mathrm{p}\right)$ is defined as an 8-point cubic spline with manually chosen points.

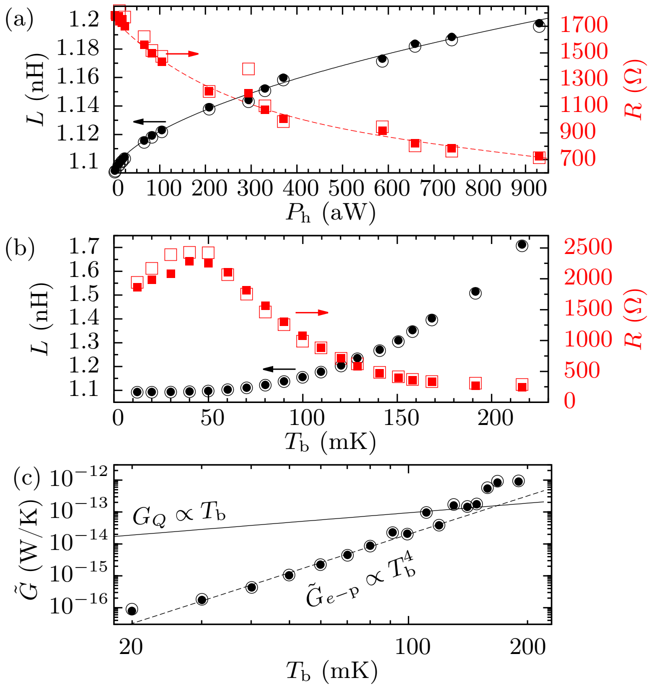


Figure S5. Same as Fig. 2, but with the additional open symbols showing the values obtained without the phenomenological correction to the fits. In addition, panel (b) shows the bath temperature dependence of $R$, instead of $\tau$.

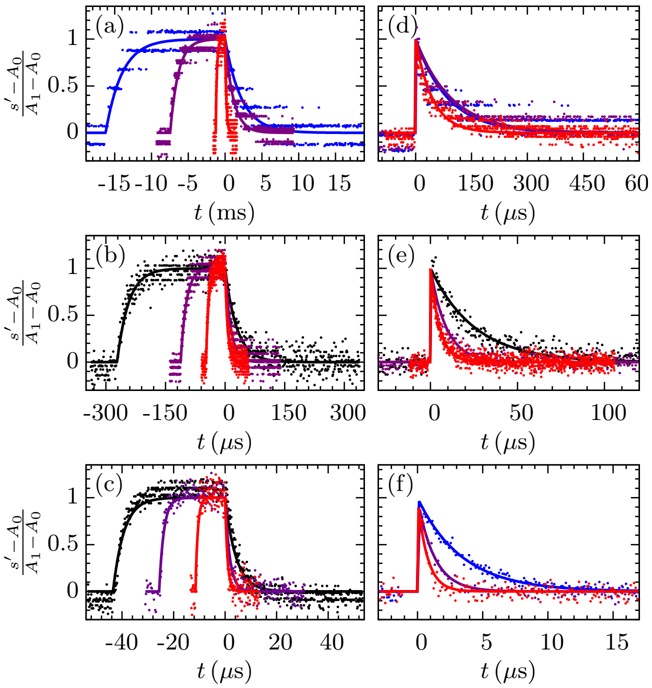


Figure S6. Time-resolved response of the normalized reflection coefficient to (a,b,c) a long and (d,e,f) a short heating pulse. The bath temperatures are (a,d) 12, 40, 70, (b,e) 100, 120, 140, (c,f) 150, 180, and 220 mK for the curves from longer to shorter time constant. The solid curves are fits to the models in Eqs. (S1) and (S2).

Including this phenomenological correction in the fits leads to the solid curves shown in Figs. 1(c), S3, and S4(a,b). The extracted fit parameters are shown in Fig. S5(a,b), with and without the phenomenological correction. Figure S5(c) also shows $\tilde{G}(T_\mathrm{b})$ with and without the correction. The agreement between the filled and open symbols in Fig. S5 confirms that the results shown in Fig. 2 are insensitive to the precise form of the phenomenological correction. We also emphasize that the correction does not affect the histograms in Fig. 4 since they do not rely on the fits.

## III. MEASUREMENT OF $\tilde{G}$

In addition to $L(T_\mathrm{b}, P_\mathrm{h} = 0)$ [Fig. 2(b)], we also measure $L(T_\mathrm{b}, P_\mathrm{h} = \delta P_\mathrm{h})$, where $\delta P_\mathrm{h}$ is small [see Fig. S4]. The differential thermal conductance $\tilde{G}$ shown in Fig. 2(c) is then computed as $\partial_{T_\mathrm{b}} L / \partial_{P_\mathrm{h}} L$, where we approximate $\partial_{P_\mathrm{h}} L$ as $[L(T_\mathrm{b}, \delta P_\mathrm{h}) - L(T_\mathrm{b}, 0)]/\delta P_\mathrm{h}$ and $\partial_{T_\mathrm{b}} L$ as the average of $[L(T_\mathrm{b}, 0) - L(T_\mathrm{b}', 0)]/(T_\mathrm{b} - T_\mathrm{b}')$ and $[L(T_\mathrm{b}'', 0) - L(T_\mathrm{b}, 0)]/(T_\mathrm{b}'' - T_\mathrm{b})$ where $T_\mathrm{b}'$ ($T_\mathrm{b}''$) is the preceding (following) data point. The ratio of the partial derivatives indeed gives $\tilde{G} = -\partial_{T_\mathrm{b}} P_{e-\mathrm{b}}(T_e, T_\mathrm{b})$, assuming that $L$ can be written as $L(T_e(T_\mathrm{b}, P_\mathrm{h}))$.

To prove the correctness of the last statement, differentiate the stationary ($\dot{T}_e = 0$) and linear response ($P_\mathrm{p} \to 0$) version of Eq. (1) with respect to $P_\mathrm{h}$ and $T_\mathrm{b}$. This gives

$$\begin{cases} 0 = -\partial_{T_e} P_{e-\mathrm{b}}(T_e, T_\mathrm{b})\, \partial_{P_\mathrm{h}} T_e + 1 \\ 0 = -\partial_{T_e} P_{e-\mathrm{b}}(T_e, T_\mathrm{b})\, \partial_{T_\mathrm{b}} T_e + \tilde{G}. \end{cases}$$

Therefore, $\tilde{G} = \partial_{T_\mathrm{b}} T_e / \partial_{P_\mathrm{h}} T_e$, which is in turn equal to $\partial_{T_\mathrm{b}} g / \partial_{P_\mathrm{h}} g$ for any smooth and monotonic function $g(T_e(T_\mathrm{b}, P_\mathrm{h}))$, including $g = L$.

## IV. MEASUREMENT OF $\tau$

We measure the thermal time constant in Fig. 2(b) using two different heating pulse patterns. In the case of a long heating pulse (open squares), the heater power remains at a small positive value $\delta P_\mathrm{h}$ from $t = -8\tau_\mathrm{g}$ to $t = 0$, and is then kept off for $16\tau_\mathrm{g}$ until the next repetition of the heating pulse. Here, $\tau_\mathrm{g}$ is the approximate thermal relaxation time determined from preliminary measurements, and $\delta P_\mathrm{h}$ is small in the sense that the resonance frequency shift caused by it is a small fraction of the linewidth. The value of $\tau_\mathrm{g}$ ($\delta P_\mathrm{h}$) varies as a function of $T_\mathrm{b}$ from 2.0 ms (−145 dBm) at 12 mK to 1.4 $\mu$s (−114 dBm) at 220 mK. We choose a probe frequency that is close to resonance and a probe power $P_\mathrm{p} \ll \delta P_\mathrm{h}$. The probe signal is turned on only between $t = -10\tau_\mathrm{g}$ and $t = 10\tau_\mathrm{g}$. The measurement is ensemble averaged over many repetitions of the pulse sequence. The number of repetitions varies from a minimum of

$2^{17}$ repetitions at 12 mK to either $2^{23}$ or $2^{24}$ for all measurements above 140 mK. Example data is shown in Fig. S6.

For the long heating pulses, we fit $\tau$ to both the rising and falling edges of the signal. Specifically, at each $T_\mathrm{b}$, we first choose a $\phi'$ that maximizes the signal $s' = \mathrm{Re}[e^{i\phi'}\Gamma(t)]$ and then fit the data to the model

$$s' = \begin{cases} A_1 + (A_\mathrm{s} - A_1)\, e^{-(t+8\tau_\mathrm{g})/\tau} & \text{if } -8\tau_\mathrm{g} < t \le 0 \\ A_0 + [s'(0) - A_0]\, e^{-\mathrm{mod}(t,24\tau_\mathrm{g})/\tau} & \text{otherwise,} \end{cases} \tag{S1}$$

with $\tau$, $A_0$, and $A_1$ as fit parameters and $A_\mathrm{s} = A_0 + (A_1 - A_0)e^{-16\tau_\mathrm{g}/\tau}$. The modulo operator in the exponent allows the inclusion of the points before the start of the heating pulse ($-10\tau_\mathrm{g} < t < -8\tau_\mathrm{g}$) in the fit.

In the case of a short heating pulse [filled squares in Fig. 2(b)], we ignore the points during the heating pulse ($-1\ \mu\mathrm{s} \le t \le 0$) and use the model

$$s' = A_0 + [A_1 - A_0]\, e^{-\mathrm{mod}(t,24\tau_\mathrm{g})/\tau}. \tag{S2}$$

The repetition period of the heating pulses is again $24\tau_\mathrm{g}$, but the value of $\tau_\mathrm{g}$ varies from 90 $\mu$s at 12 mK to 1.4 $\mu$s at 220 mK. That is, $\tau_\mathrm{g}$ approximately follows the filled, rather than the open, squares in Fig. 2(b). The probe signal is turned on between $t = -2\tau_\mathrm{g}$ and $t = 18\tau_\mathrm{g}$. The heater power $\delta P_\mathrm{h}$ varies between $-120$ dBm and $-112$ dBm and the number of averages between $2^{22}$ and $2^{24}$. The heater power is larger than in the case of the long heating pulses in order to make the maximum change in the resonance frequency similar.

We note that we measured the thermal relaxation time in a separate cooldown, with minor differences in the setup compared to Fig. S1. However, we also measured the response to a long heating pulse in the original cooldown and obtained results in good agreement with the data shown here.

## V. HEAT CAPACITY

In the main text, we use the product $\tau\tilde{G}$ as an estimate of $C_e = \tau\partial_{T_e}P_{e-\mathrm{b}}$ in the high-temperature limit, i.e., when $T_e \approx T_\mathrm{b}$. This relies on replacing $\partial_{T_e}P_{e-\mathrm{b}}$ by $\tilde{G}$. This is justified because $P_{e-\mathrm{b}}$ must vanish in thermal equilibrium, and hence, $-\partial_{T_\mathrm{b}}P_{e-\mathrm{b}}(T_e,T_\mathrm{b})$ must equal $\partial_{T_e}P_{e-\mathrm{b}}(T_e,T_\mathrm{b})$ for any $T_e = T_\mathrm{b}$. Even for $T_e > T_\mathrm{b}$, $\tilde{G}(T) = -\partial_{T_\mathrm{b}}P_{e-\mathrm{b}}(T_e, T_\mathrm{b} = T)$ equals $\partial_{T_e}P_{e-\mathrm{b}}(T_e = T, T_\mathrm{b})$ provided that the net heat flow $P_{e-\mathrm{b}}(T_e,T_\mathrm{b})$ can be written as $P_{e\to\mathrm{b}}(T_e) - P_{\mathrm{b}\to e}(T_\mathrm{b})$. Again, this is true because $P_{e\to\mathrm{b}}$ and $P_{\mathrm{b}\to e}$ must in fact be the same function so that $P_{e-\mathrm{b}}$ vanishes when $T_e = T_\mathrm{b}$.

In the main text, we also state that, above 100 mK, $\tau\tilde{G} \approx \gamma V_0 T_\mathrm{b}$, with $\gamma V_0 = 8\ \mathrm{aJ/K^2}$. Figure S7 demonstrates this in more detail. Note that the extracted value of $\gamma$ is only about a fifth larger than expected based on a naive weighted average of the electronic specific heats of Au (60 %) and Pd (40 %).

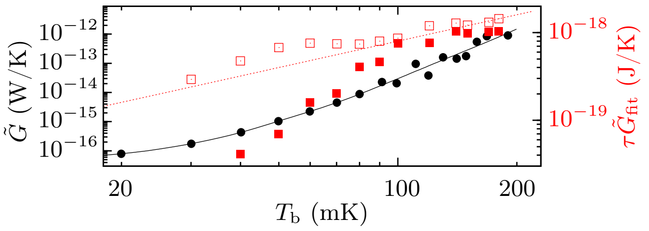


Figure S7. Measured differential thermal conductance $\tilde{G}$ (circles), a phenomenological fit $\tilde{G}_\mathrm{fit}$ (solid line), and the product $\tau\tilde{G}_\mathrm{fit}$ (squares) as functions of bath temperature. The product $\tau\tilde{G}_\mathrm{fit}$ is a good estimate of the heat capacity at $T_\mathrm{b} > 100$ mK, where the system is described by a single thermal time constant and $T_e \approx T_b$. The open and filled squares correspond to the open and filled squares in Fig. 2(b), respectively. The dashed line shows a linear fit $\gamma V_0 T_e$, with $\gamma V_0 = 8\ \mathrm{aJ/K^2}$.

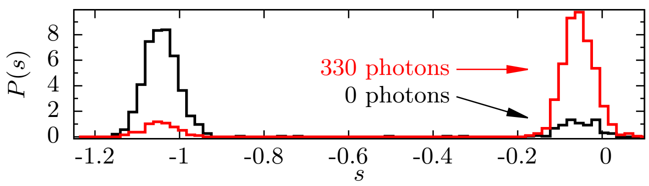


Figure S8. Same as Fig. 4(b), but for a 1.9 zJ heat pulse and $t_s = 3.8\ \mu$s.

## VI. NUMERICAL MODEL FOR BISTABILITY

To produce Fig. 3(b), we first solve for the stationary solutions of Eq. (3) numerically on an $f_\mathrm{p} - P_\mathrm{p}$ grid of $208 \times 161$ points. This requires evaluating $|\Gamma(\Delta,\omega)|^2$, which we determine from the phenomenological fit functions shown in Fig. 2(a). They give $L(\Delta)$ and $R(\Delta)$, which we in turn use in the simplified circuit model for predicting $\Gamma = (Z_\mathrm{L} - Z_0)/(Z_\mathrm{L} + Z_0)$. We find the stationary $\Delta$ solutions at each $f_\mathrm{p}$ and $P_\mathrm{p}$ by simply computing the value of the right-hand side of Eq. (3) on a $\Delta$ grid of 4001 points between 0 and 200 aW. This method is robust in finding all zero crossings, i.e., either one or three values of $\Delta$ that satisfy Eq. (3) in a stationary state at a given $f_\mathrm{p}$ and $P_\mathrm{p}$. This is sufficient for determining the boundary of the bistable region shown in Fig. 3(b).

In order to determine $\chi$, we differentiate the stationary ($\dot{\Delta} = 0$) version of Eq. (3) with respect to $P_\mathrm{h}$. This leads to

$$\chi = \left(1 + P_\mathrm{p}\frac{\partial|\Gamma(\Delta,\omega)|^2}{\partial\Delta}\right)^{-1}.$$

To determine $\partial_\Delta|\Gamma(\Delta,\omega)|^2$, we evaluate $|\Gamma(\Delta,\omega)|^2$ at the $\Delta(P_\mathrm{p},\omega)$ solved above and at $\Delta + \delta\Delta$, where $\delta\Delta \ll \Delta$ and $\left||\Gamma(\Delta,\omega)|^2 - |\Gamma(\Delta+\delta\Delta,\omega)|^2\right| \ll 1$.

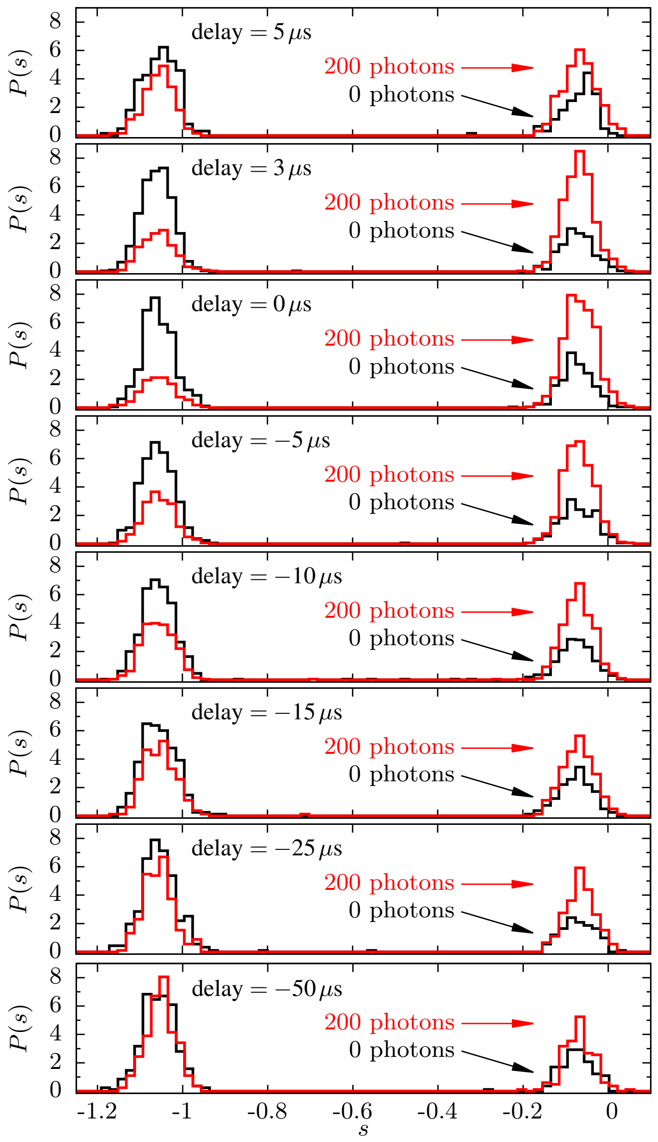


Figure S9. Same as Fig. 4(b), but for a time delay of 5, 3, 0, −5, −10, −15, −25, or −50 $\mu$s from the start of the probe pulse to the start of the heat pulse. The corresponding fidelities are 0.24, 0.44, 0.46, 0.37, 0.29, 0.21, 0.21, and 0.11. The number of samples used for the histograms varies between 312 and $10^3$.

## VII. ADDITIONAL SINGLE-SHOT HISTOGRAMS

Figure S8 shows the histogram for a 330 photon heat pulse. The corresponding readout fidelity is $F = 0.75$, as mentioned in the main text. Note that $t_s$ is tuned in each panel in Fig. 4 and Fig. S8 so that $P(s > -0.25|\text{no heat pulse})$ is approximately equal to $P(s \leq -0.25|\text{heat pulse})$. This maximizes the fidelity for a given pulse energy, and therefore makes a comparison of $F$ to $\bar{F}$ meaningful.

Figure S9 illustrates the sensitivity of the detector to varying the relative timing of the heat and probe pulses. The optimal delay between the pulses is near zero, which is why we choose a small (1 $\mu$s) delay in the pulse sequence shown in Fig. 4. As expected, delaying the heat pulse by more than $t_s$ leads to rapid deterioration of the fidelity. On the other hand, the fidelity decays more slowly when the delay becomes more negative, i.e., when the heat pulse precedes the probe. This is expected since a negative delay $t_d$ should have roughly the same effect as decreasing the magnitude of the heat pulse by a factor of $e^{-|t_d|/\tau(T_e^\star)}$, where $\tau(T_e^\star)$ is the thermal relaxation time at the elevated electron temperature $T_e^\star$ just after the absorption of the heat pulse. The observed $t_d$ dependence of $F$ is consistent with $\tau(T_e^\star) \approx 90$ $\mu$s estimated from Fig. 2(b).

* joonas.govenius@aalto.fi
